# Supplementary material for: Connecting Gaits in Energetically Conservative Legged Systems
Source: arXiv:2203.00782 source file (2024-02-09)
Supplement: Supplementary file 1 [file AppendixSLIP.tex]

\Max{\section{Appendix}
\subsection{SLIP Model Dynamics}
The mass matrix in the one legged hopper is given by
\small
\begin{align}\label{eq:MassMatrixSLIP}
\mat M(\vec q)&=\dfrac{\partial^2 T}{\partial \dot{\vec{q}}^2}\\
&=\begin{bmatrix}[1.3] m_o & 0 & m_\mathrm{f} l C & m_\mathrm{f} l C & m_\mathrm{f} S\\
0&m_o&m_\mathrm{f} lS&m_\mathrm{f} lS&-m_\mathrm{f} C\\
m_\mathrm{f} l C&m_\mathrm{f} lS&m_\mathrm{f} l^2+\Theta_\mathrm{t}& m_\mathrm{f} l^2&0\\
m_\mathrm{f} l C&m_\mathrm{f} lS&m_\mathrm{f} l^2& m_\mathrm{f} l^2&0\\
m_\mathrm{f} S&-m_\mathrm{f} C&0&0&m_\mathrm{f}
\end{bmatrix},\notag 
\end{align}
\normalsize
and the inertial vector takes the form
\small
\begin{equation}
    \vec h(\vec q,\dot{\vec q})= \begin{bmatrix}[1.3] m_\mathrm{f}\dot \gamma\left(Sl\dot \gamma-2C\dot{l}\right)\\
    -m_\mathrm{f} C l \dot \gamma^2-2m_\mathrm{f}S\dot{l}\dot \gamma-m_o g\\
    -m_\mathrm{f} l \left(S g +2\dot{l}\dot \gamma\right)\\
    -m_\mathrm{f} l \left(S g +2\dot{l}\dot \gamma\right)\\
    m_\mathrm{f} \left(l\dot \gamma^2 +C g\right)
    \end{bmatrix},
\end{equation}
\normalsize
where we used again the abbreviations \mbox{$C=\cos(\varphi+\alpha)$}, \mbox{$S=\sin(\varphi+\alpha)$} and \mbox{$\dot \gamma = \dot{\varphi}+\dot{\alpha}$}. During flight phase, the generalized accelerations can be explicitly stated, with \eqref{eq:lambdaF_new} and \eqref{eq:legswingfreq}, as
\small
\begin{equation}
   \ddot{\vec q}_\mathrm{F} =
   \begin{bmatrix}[2.5]
   \ddot x_\mathrm{F}\\\ddot y_\mathrm{F}\\ \ddot \varphi_\mathrm{F}\\ \ddot \alpha_\mathrm{F}\\ \ddot l_\mathrm{F}
   \end{bmatrix} =
   \begin{bmatrix}[2.5] m_\mathrm{f}\dfrac{C \omega_\mathrm{swing}^2 m_o l_o^2\alpha -Sl\hat{\lambda}_\mathrm{F}}{l\,m_o\,m_\mathrm{t}}\\ 
   -g+m_\mathrm{f}\dfrac{S \omega_\mathrm{swing}^2 m_o l_o^2\alpha+Cl\hat{\lambda}_\mathrm{F}}{l\,m_{0}\,m_{t}}\\ m_\mathrm{f}\dfrac{\omega_\mathrm{swing}^2l_o^2}{\theta_\mathrm{t}}\alpha\\ -\dfrac{2}{l}\dot \gamma\dot{l}-\omega_\mathrm{swing}^2 l_o^2 \left(\dfrac{m_o}{m_\mathrm{t}l^2}+\dfrac{m_\mathrm{f}}{\theta_\mathrm{t}}\right)\alpha\\ l \dot \gamma^2+\dfrac{\hat{\lambda }_\mathrm{F}}{m_\mathrm{t}}\end{bmatrix},
\end{equation}
\normalsize
where the flight constraint $l-l_o=0$ yields $\dot l \equiv \ddot l \equiv 0$ and thus
\begin{equation}
    \hat{\lambda}_\mathrm{F}=-m_\mathrm{t} l_o \dot \gamma^2.
\end{equation}
Similar for the stance phase, with \eqref{eq:lambdaS_new} and \eqref{eq:legswingfreq}, the generalized accelerations are:
\small
\begin{equation}
   \ddot{\vec q}_\mathrm{S}  = \begin{bmatrix}[2.5] m_\mathrm{f}\dfrac{C\omega_\mathrm{swing}^2l_o^2}{m_\mathrm{t}l}\alpha-S \dfrac{F_\mathrm{l}}{m_\mathrm{t}}\\
   m_\mathrm{f}\dfrac{S\omega_\mathrm{swing}^2l_o^2}{m_\mathrm{t}l}\alpha-g+C \dfrac{F_\mathrm{l}}{m_\mathrm{t}}\\ m_\mathrm{f}\dfrac{\omega_\mathrm{swing}^2l_o^2}{\theta_\mathrm{t}}\alpha\\ \ddot \alpha_\mathrm{F}+[C~S] \cdot \dfrac{\hat{\vec \lambda}_{\mathrm{S}}}{m_o l} \\
   l \dot \gamma^2+\dfrac{F_\mathrm{l}}{ m_\mathrm{t}}+[S~-C] \cdot \dfrac{\hat{\vec \lambda}_{\mathrm{S}}}{m_o} \end{bmatrix}.
\end{equation}
\normalsize
The auxiliary contact forces during stance follow from \eqref{eq:ConstraintS} and \eqref{eq:lambdaS_new}:
\begin{equation}
\hat{\vec \lambda}_{\mathrm{S}} =
    \begin{bmatrix}
        \dfrac{C}{l}\omega_\mathrm{swing}^2 m_o l_o^2\alpha\\
        m_o g+\dfrac{S}{l}\omega_\mathrm{swing}^2 m_o l_o^2\alpha
    \end{bmatrix}.
\end{equation}
Note, the foot mass $m_\mathrm{f}$ can be arbitrary and does not cause any dynamical singularities. For $m_f=0$ ($\varepsilon\to 0$), we get the same dynamics as reported in \cite{gan2018}.}
